# Supplementary material for: Inversion in a four terminal superconducting device on the quartet line: II. Quantum dot and Floquet theory
Source: arXiv:2008.01983 ancillary file (2020-11-16)
Supplement: Supplementary file 1 [file revised_supplemental_material_final_paperII.pdf]

# Inversion in a four-terminal superconducting device on the quartet line: II. Quantum dot and Floquet theory Supplemental Material

Régis Mélin[1] and Benoît Douçot[2]

[1]*Univ. Grenoble-Alpes, CNRS, Grenoble INP, Institut NEEL, 38000 Grenoble, France*

[2]*Laboratoire de Physique Théorique et Hautes Energies, Sorbonne Université and CNRS UMR 7589, 4 place Jussieu, 75252 Paris Cedex 05, France*

The supplemental Material contains the technical details of the calculations.

The Supplemental Material is organized as the following. Section I contains the necessary technical details about the multilevel quantum dot model. Section II contains calculations of the inversion in the $V=0^+$ adiabatic limit. Section III discusses the robustness of the inversion against changing the value of $\gamma/\Delta$.

## I. MULTILEVEL QUANTUM DOT

In this section, we provide the model of multilevel quantum dot which is mentioned in section III E of the paper, and used in section VI of the paper.

The Hamiltonian of a quantum dot with $M$ levels is given by

$$\mathcal{H}_{dot} = \sum_{\alpha=1}^{M} E_\alpha d^+_{\alpha,\sigma} d_{\alpha,\sigma} \tag{1}$$

and the coupling to the leads is given by

$$\mathcal{H}_{tunnel} = \sum_{j,\alpha,\mathbf{k}} \left( J_{j\alpha} e^{-is_j\omega_0 t} c^+_{j,\mathbf{k},\sigma} d_{\alpha,\sigma} + J^*_{j\alpha} e^{is_j\omega_0 t} d^+_{\alpha,\sigma} c_{j,\mathbf{k},\sigma} \right). \tag{2}$$

The Floquet-Lippmann-Schwinger equations are the following:

$$\left(E(j,\mathbf{k}) + m\omega_0 - E_\alpha + i\eta\right) u_m(\alpha; j\mathbf{k}) = \sum_{i=1}^{N} J^*_{i\alpha} \int \frac{d^3\mathbf{k}'}{(2\pi)^3} u_{m+s_i}(i\mathbf{k}'; j\mathbf{k}) + J^*_{j\alpha} \delta_{m,-s_j} x(j,\mathbf{k}) e^{i\varphi_j/2} \tag{3}$$

$$\left(E(j,\mathbf{k}) + m\omega_0 + E_\alpha + i\eta\right) v_m(\alpha; j\mathbf{k}) = -\sum_{i=1}^{N} J_{i\alpha} \int \frac{d^3\mathbf{k}'}{(2\pi)^3} v_{m-s_i}(i\mathbf{k}'; j\mathbf{k}) - J_{j\alpha} \delta_{m,s_j} y(j,\mathbf{k}) e^{-i\varphi_j/2} \tag{4}$$

$$\big(E(j,\mathbf{k}) + m\omega_0 - \varepsilon(i\mathbf{k}') + i\eta\big) u_m(i\mathbf{k}'; j\mathbf{k}) = \Delta_i v_m(i\mathbf{k}'; j\mathbf{k}) + \sum_\alpha J_{i\alpha} u_{m-s_i}(\alpha; j\mathbf{k}) \tag{5}$$

$$\big(E(j,\mathbf{k}) + m\omega_0 + \varepsilon(i\mathbf{k}') + i\eta\big) v_m(i\mathbf{k}'; j\mathbf{k}) = \Delta^*_i u_m(i\mathbf{k}'; j\mathbf{k}) - \sum_\alpha J^*_{i\alpha} v_{m+s_i}(\alpha; j\mathbf{k}). \tag{6}$$

In these equations, $\varepsilon(i\mathbf{k}')$ denotes the energy (subtracted by the chemical potential) of a single quasiparticle of momentum $\mathbf{k}'$) created above the normal state in reservoir $i$. In the absence of tunnel couplings between the reservoirs and the dot, quasi-particle creation operators in reservoir $j$ have the form $\gamma^+_{j,\mathbf{k},\sigma} = x(j,\mathbf{k}) e^{i\varphi_j/2} c^+_{j,\mathbf{k},\sigma} + e^{-i\varphi_j/2} y(j,\mathbf{k}) c_{j,-\mathbf{k},-\sigma}$, with $x(j,\mathbf{k})$ and $y(j,\mathbf{k})$ given by BCS theory. In the presence of time-periodic tunnel couplings, we look for Floquet solutions $\Gamma^+_{j,\mathbf{k},\sigma}(t)$ of the time dependent Bogoliubov-De Gennes equations, which reduce to $\Gamma^+_{j,\mathbf{k},\sigma}(t) = e^{-iE_{j,\mathbf{k}}t} \gamma^+_{j,\mathbf{k},\sigma}$ in the limit of vanishing tunnel coupling. Floquet Ansatz means that we can write $\Gamma^+_{j,\mathbf{k},\sigma}(t) = e^{-iE_{j,\mathbf{k}}t} \chi^+_{j,\mathbf{k},\sigma}(t)$, where the operator $\chi^+_{j,\mathbf{k},\sigma}(t)$ is periodic in time. Expanding it in Fourier series, the corresponding coefficients are operators $\chi^+_m(j\mathbf{k})$, where the integer $m$ labels the different harmonics. The complete expression of $\chi^+_m(j\mathbf{k})$ involves amplitudes $u_m(\alpha; j\mathbf{k})$, $v_m(\alpha; j\mathbf{k})$ on the dot, and $u_m(i\mathbf{k}'; j\mathbf{k})$, $v_m(i\mathbf{k}'; j\mathbf{k})$ on reservoir $i$ . These four sets of amplitudes are determined by the above coupled inhomogeneous linear equations, which have the same form as the Lippmann-Schwinger equations used to determine scattering states in quantum scattering theory[1]. Note that the scattering formalism for Floquet states has been developed in the context of ac transport through non superconducting quantum circuits by several groups before[2,3]. In the case of a single level quantum dot coupled to several superconducting reservoirs, more details on the derivation of the above equations are provided in the Supplemental Material of Ref. 4.

Using now the last two Eqs. (5)-(6), we eliminate the amplitudes in the leads, which leads to

$$(E+m\omega_0-E_\alpha+i\eta)\,u_m(\alpha;j\mathbf{k})-\sum_{i=1}^{N}\sum_{\beta=1}^{M}J^*_{i\alpha}g^{(i)}_{1,1}(E+(m+s_i)\omega_0)J_{i\beta}u_m(\beta;j\mathbf{k}) \tag{7}$$

$$+\sum_{i=1}^{N}\sum_{\beta=1}^{M}J^*_{i\alpha}g^{(i)}_{1,2}(E+(m+s_i)\omega_0)J^*_{i\beta}v_{m+2s_i}(\beta;j\mathbf{k})=J^*_{j\alpha}\delta_{m,-s_j}x(j\mathbf{k})e^{i\varphi_j/2}$$

$$(E+m\omega_0+E_\alpha+i\eta)\,v_m(\alpha;j\mathbf{k})-\sum_{i=1}^{N}\sum_{\beta=1}^{M}J_{i\alpha}g^{(i)}_{2,2}(E+(m-s_i)\omega_0)J^*_{i\beta}v_m(\beta;j\mathbf{k}) \tag{8}$$

$$+\sum_{i=1}^{N}\sum_{\beta=1}^{M}J_{i\alpha}g^{(i)}_{2,1}(E+(m-s_i)\omega_0)J_{i\beta}u_{m-2s_i}(\beta;j\mathbf{k})=-J_{j\alpha}\delta_{m,s_j}y(j\mathbf{k})e^{-i\varphi_j/2}.$$

Thus, we obtain a 1D effective Hamiltonian with $2M$ internal states. Then, it is possible to reduce to only two internal states under the specific assumption of factorization of the tunneling amplitudes: $J_{i,\alpha}=J_i f_\alpha$. Then, let us define $\tilde{d}_\sigma=\sum_\alpha f_\alpha d_{\alpha\sigma}$, $\tilde{d}^+_\sigma=\sum_\alpha f^*_\alpha d^+_{\alpha\sigma}$. Then, $\{\tilde{d}_\sigma,\tilde{d}^+_\sigma\}=1$ if $\sum_\alpha|f_\alpha|^2=1$, and Eq. (2) becomes

$$\mathscr{H}_{tunnel}=\sum_{j=1}^{N}\left(J_j e^{-is_j\omega_0 t}c^+_{j,\mathbf{k},\sigma}\tilde{d}_\sigma+J^*_j e^{is_j\omega_0 t}\tilde{d}^+_\sigma c_{j,\mathbf{k},\sigma}\right). \tag{9}$$

Then, we define

$$r_m(j\mathbf{k})\equiv\sum_{\beta=1}^{M}f_\beta u_m(\beta;j\mathbf{k}) \tag{10}$$

$$s_m(j\mathbf{k})\equiv\sum_{\beta=1}^{M}f^*_\beta v_m(\beta;j\mathbf{k}). \tag{11}$$

Applying $\sum_{\alpha=1}^{M}f_\alpha/(E+m\omega_0-E_\alpha+i\eta)$ on Eq. (7) and $\sum_{\alpha=1}^{M}f^*_\alpha/(E+m\omega_0+E_\alpha+i\eta)$ on Eq. (8) leads to

$$r_m(j\mathbf{k})-g^{(dot,p)}(E+m\omega_0)\sum_{i=1}^{N}\left(J^*_i g^{(i)}_{1,1}(E+(m+s_i)\omega_0)J_i\right)r_m(j\mathbf{k}) \tag{12}$$

$$+g^{(dot,p)}(E+m\omega_0)\sum_{i=1}^{N}J^*_i g^{(i)}_{1,2}(E+(m+s_i)\omega_0)J^*_i s_{m+2s_i}(j\mathbf{k})=J^*_j g^{(dot,p)}(E+m\omega_0)\delta_{m,-s_j}x(j\mathbf{k})e^{i\varphi_j/2}$$

$$s_m(j\mathbf{k})-g^{(dot,h)}(E+m\omega_0)\sum_{i=1}^{N}\left(J_i g^{(i)}_{2,2}(E+(m-s_i)\omega_0)J^*_i\right)s_m(j\mathbf{k}) \tag{13}$$

$$+g^{(dot,h)}(E+m\omega_0)\sum_{i=1}^{N}J_i g^{(i)}_{2,1}(E+(m-s_i)\omega_0)J_i r_{m-2s_i}(j\mathbf{k})=-J_j g^{(dot,h)}(E+m\omega_0)\delta_{m,s_j}y(j\mathbf{k})e^{-i\varphi_j/2},$$

where we used

$$g^{(dot,p)}(E)=\sum_{\alpha=1}^{M}\frac{|f_\alpha|}{E-E_\alpha+i\eta} \tag{14}$$

$$g^{(dot,h)}(E)=\sum_{\alpha=1}^{M}\frac{|f_\alpha|}{E+E_\alpha+i\eta}. \tag{15}$$

Eqs. (12) and (13) are implemented numerically in the paper.

## II. INVERSION IN THE $V=0^+$ ADIABATIC LIMIT

In this section, we investigate the conditions for emergence of inversion in the $V=0^+$ adiabatic limit.

### A. Analytical results

We demonstrate now that the inversion can be obtained in the small-$\Phi/\Phi_0$ limit, *i.e.* $I_c(\Phi/\Phi_0)$ increases with $\Phi/\Phi_0$. Inversion can also be obtained between $\Phi/\Phi_0=0$ and $\Phi/\Phi_0=1/2$, *i.e.* $I_c(0)<I_c(1/2)$.

The two equilibrium ABS energies deduced from the $2\times 2$ Hamiltonian in the infinite-gap limit are given by $\pm|\Gamma(k)|$, with

$$\Gamma(k)=\Gamma_a e^{i(\varphi_a+k)}+\Gamma_b e^{i(\varphi_b-k)}+\Gamma_{c,1}e^{i\varphi_c}+\Gamma_{c,2}e^{i(\varphi_c+\Phi)}, \tag{16}$$

where $k$ is defined by Eqs. (3)-(7) in the paper. Averaging over the "fast" phase variable $k$ yields the following form for

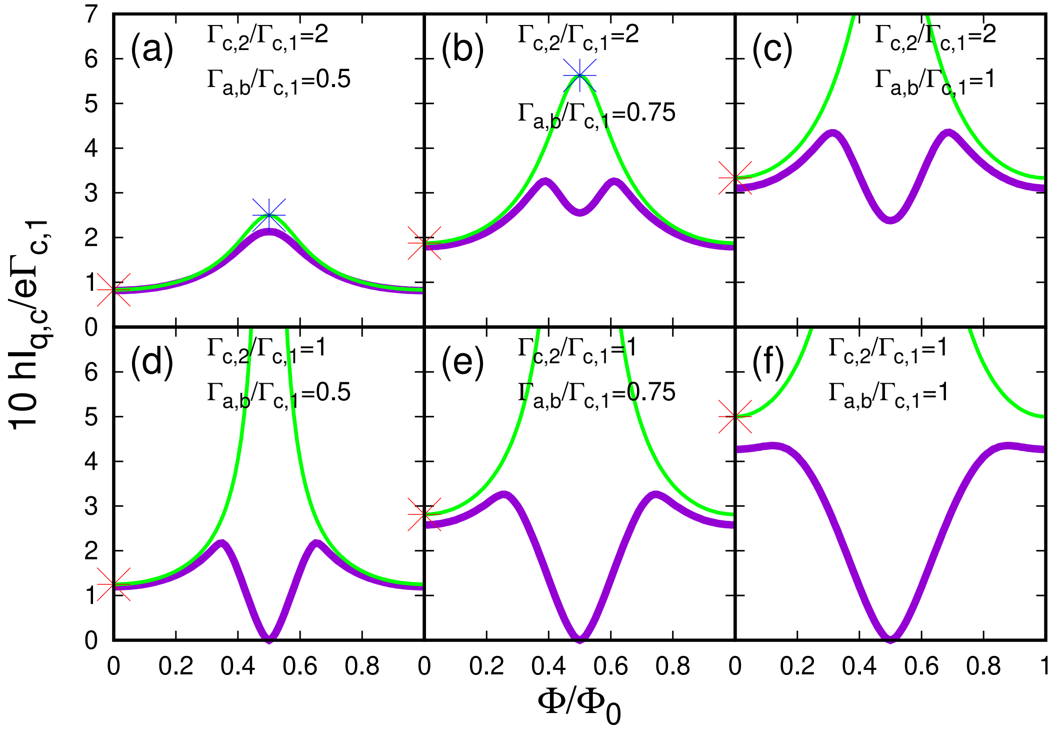


FIG. 1. *Flux-*$\Phi/\Phi_0$ *sensitivity of the critical current* $I_c(\Phi/\Phi_0)$ *if both the infinite-gap and the* $V=0^+$ *adiabatic limits are simultaneously taken.* The magenta and green lines compared the exact numerical result to the approximation given by Eq. (29) respectively. The red cross and the blue star show this approximation in the limit $\Phi/\Phi_0=0$ and $\Phi/\Phi_0=1/2$ respectively. The value $\Gamma_{c,1}/\Gamma_{c,2}=2$ and $\Gamma_{c,1}/\Gamma_{c,2}=1$ are used on panels (a,b,c) and (d,e,f) respectively. The values $\Gamma_a/\Gamma_{c,1}=(0.5,0.75,1)$ are used on panels (a,b,c) respectively, as well as on panels (d,e,f).

the sum of the currents $I_{c,1}+I_{c,2}$ transmitted into the grounded loop $S_c$:

$$I_{S_c}=-\frac{2e}{\hbar}\frac{\partial}{\partial\varphi_c}\langle E_{ABS}\rangle_k, \tag{17}$$

where $\langle\ldots\rangle_k$ is defined as

$$\langle E_{ABS}\rangle_k=\int_0^{2\pi}\frac{dk}{2\pi}\,|\Gamma(k)|\,. \tag{18}$$

We assume now that the superconducting leads $S_{c,1}$ and $S_{c,2}$ are strongly coupled to the dot, and that $S_a$, $S_b$ are weakly coupled. This assumption of asymmetric coupling to the leads allows for an expansion of the ABS energy $E_{ABS}=|\Gamma(k)|$ in the small parameters $\Gamma_a/\Gamma_{c,1}\ll 1$, $\Gamma_b/\Gamma_{c,1}\ll 1$, $\Gamma_a/\Gamma_{c,2}\ll 1$ and $\Gamma_b/\Gamma_{c,2}\ll 1$, supposed to take small values within a similar range.

More specifically, we take the square modulus of Eq. (16) according to

$$|\Gamma(k)|^2=\mathscr{D}(\Phi/\Phi_0)\,(1+a+b+\ldots)\,, \tag{19}$$

where $a=\sum_{i=1}^4 a_i$, with

$$a_1=\frac{2\Gamma_a\Gamma_{c,1}}{\mathscr{D}(\Phi/\Phi_0)}\cos\left(\varphi_a-\varphi_c+k\right) \tag{20}$$

$$a_2=\frac{2\Gamma_a\Gamma_{c,2}}{\mathscr{D}(\Phi/\Phi_0)}\cos\left(\varphi_a-\varphi_c+\Phi+k\right) \tag{21}$$

$$a_3=\frac{2\Gamma_b\Gamma_{c,1}}{\mathscr{D}(\Phi/\Phi_0)}\cos\left(\varphi_b-\varphi_c-k\right) \tag{22}$$

$$a_4=\frac{2\Gamma_b\Gamma_{c,2}}{\mathscr{D}(\Phi/\Phi_0)}\cos\left(\varphi_b-\varphi_c-\Phi+k\right), \tag{23}$$

and

$$\mathscr{D}(\Phi/\Phi_0)=\Gamma_{c,1}^2+\Gamma_{c,2}^2+2\Gamma_{c,1}\Gamma_{c,2}\cos\Phi \tag{24}$$

$$b=\frac{\Gamma_a^2+\Gamma_b^2}{\mathscr{D}(\Phi/\Phi_0)}+\frac{2\Gamma_a\Gamma_b}{\mathscr{D}(\Phi/\Phi_0)}\cos\left(\varphi_a-\varphi_b+2k\right). \tag{25}$$

The expansion

$$\sqrt{1+a+b+\ldots}\simeq 1+\frac{a}{2}+\frac{1}{2}\left(b-\frac{a^2}{4}\right)+\ldots \tag{26}$$

leads to

$$\langle|\Gamma|\rangle_k=\sqrt{\mathscr{D}(\Phi/\Phi_0)}\left\{1+\frac{\Gamma_a^2+\Gamma_b^2}{2\mathscr{D}(\Phi/\Phi_0)}-\frac{1}{8}\langle a^2\rangle_k+\ldots\right\}. \tag{27}$$

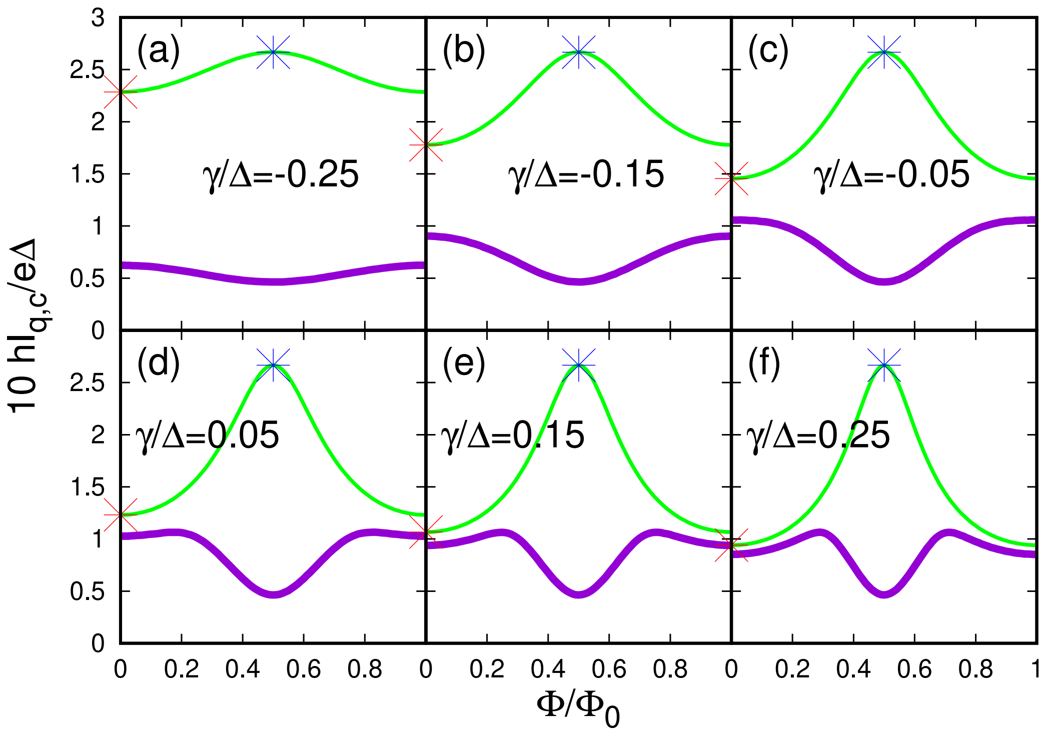


FIG. 2. The same as figure 1, but now the coupling constants are given by Eqs. (25)-(28) in the text of the paper, *i.e.* they are the same as those used in the finite bias voltage calculations. The following values of $\gamma/\Delta$ are used $\gamma/\Delta = -0.25$ (panel a), $\gamma/\Delta = -0.15$ (panel b), $\gamma/\Delta = -0.05$ (panel c), $\gamma/\Delta = 0.05$ (panel d), $\gamma/\Delta = 0.15$ (panel e) and $\gamma/\Delta = 0.25$ (panel f).

A straightforward calculation of the $k$-averaged $\langle a_i a_j \rangle_k$ (with $i,j = 1,...,4$) leads to

$$-\frac{\partial \langle |\Gamma| \rangle}{\partial \varphi_c} = \frac{\Gamma_a \Gamma_b}{\sqrt{\mathscr{D}(\Phi/\Phi_0)}} \sin \varphi_q. \tag{28}$$

The resulting critical current is the following:

$$I_c(\Phi/\Phi_0) = \frac{2e}{\hbar} \frac{\Gamma_a \Gamma_b}{\sqrt{\mathscr{D}(\Phi/\Phi_0)}}, \tag{29}$$

where $\mathscr{D}(\Phi/\Phi_0)$ is given by Eq. (24).

Combining Eq. (24) to Eq. (29) leads to the following small-$\Phi$ approximation to the critical current $I_c(\Phi/\Phi_0)$:

$$I_c \simeq \frac{2e}{\hbar} \frac{\Gamma_a \Gamma_b}{\Gamma_{c,1} + \Gamma_{c,2}} \left\{ 1 + \frac{\Gamma_{c,1} \Gamma_{c,2}}{2 \left( \Gamma_{c,1} + \Gamma_{c,2} \right)^2} \Phi^2 \right\}. \tag{30}$$

Inversion in the small-$\Phi$ limit is obtained, namely, the quartet critical current $I_c$ increases with $\Phi$ at small $\Phi$.

We deduce the following from Eqs. (24) and (29):

$$I_c(0) \simeq \frac{2e}{\hbar} \frac{\Gamma_a \Gamma_b}{\Gamma_{c,1} + \Gamma_{c,2}} \tag{31}$$

$$I_c(1/2) \simeq \frac{2e}{\hbar} \frac{\Gamma_a \Gamma_b}{|\Gamma_{c,1} - \Gamma_{c,2}|}, \tag{32}$$

where Eq. (31) coincides with the $\Phi = 0$ limit of the previous Eqs. (29) and (30).

Eq. (32) implies that the perturbation in small-$\Gamma_a$ and $\Gamma_b$ converges on the condition that $|\Gamma_{c,1} - \Gamma_{c,2}|$ is large compared to $\Gamma_a, \Gamma_b$. Within this assumption about the validity of the approximation around $\Phi/\Phi_0 \simeq 1/2$, Eqs. (31) and (32) imply "inverted behavior of $I_c(\Phi/\Phi_0)$ between $\Phi/\Phi_0 = 0$ and $\Phi/\Phi_0 = 1/2$, namely $I_c(0) < I_c(1/2)$ in Eqs. (31) and (32).

### B. Numerical results

Figures 1a, b and c above correspond to $\Gamma_{c,2}/\Gamma_{c,1} = 2$, *i.e.* to asymmetric coupling between the quantum dot and each of the two $S_{c,1}$ and $S_{c,2}$, being the contact points of both arms of the loop on the quantum dot. Panel d, e, f of figure 1 correspond to the loop symmetrically coupled on the dot, with $\Gamma_{c,2}/\Gamma_{c,1} = 1$. Identical values of $\Gamma_a = \Gamma_b \equiv \Gamma_{a,b}$ are used on all panels. The ratio $\Gamma_{a,b}/\Gamma_{c,1}$ increases from $\Gamma_{a,b}/\Gamma_{c,1} = 0.5$ (panel a) to $\Gamma_{a,b}/\Gamma_{c,1} = 0.75$ (panel b) and next to $\Gamma_{a,b}/\Gamma_{c,1} = 1$ (panel c). The same values of $\Gamma_{a,b}/\Gamma_{c,1}$ are used on panels d, e and f respectively.

All panels of figure 1 show the dependence of the critical current $I_c(\Phi/\Phi_0)$ (normalized to $e\Gamma_{c,1}/h$) on $y$-axis as a function of the reduced flux $\Phi/\Phi_0$ on $x$-axis. The numerically exact calculation in the $V = 0^+$ adiabatic limit is shown as magenta lines. The green lines show the $\Phi/\Phi_0$-dependence of the low-$\Gamma_{a,b}$ analytical approximation [see Eq. (29)], extrapolated to general values of $\Gamma_a$ and $\Gamma_b$, for which Eq. (29)

can be a bad approximation. The red cross are the value of this approximation at $\Phi/\Phi_0 = 0$ [see Eq. (31)], and the blue stars correspond to Eq. (31) for $\Phi/\Phi_0 = 1/2$, see Eq. (32). The blue stars are not visible on panels c, d, e, and f, because they are outside the frame of these panels, above the $y$-axis range.

On figure 1, the approximation given by Eq. (29) (shown as a green line) is the closest to the numerically exact calculation (magenta line) for the smallest values of $\Gamma_{c,1}/\Gamma_{c,2}$ and also for the smallest $\Gamma_{a,b}/\Gamma_{c,1}$. Namely, as $\Gamma_{a,b}/\Gamma_{c,1}$ increases from $\Gamma_{a,b}/\Gamma_{c,1} = 0.5$ (panel a) to $\Gamma_{a,b}/\Gamma_{c,1} = 0.75$ (panel b) and next to $\Gamma_{a,b}/\Gamma_{c,1} = 1$ (panel c), we see that Eq. (1) (green line) crosses over from being an excellent approximation if $\Gamma_{a,b}/\Gamma_{c,1} = 0.5$ (panel a) to showing important deviations as $\Gamma_{a,b}/\Gamma_{c,1}$ is increased to $\Gamma_{a,b}/\Gamma_{c,1} = 0.75$ (panel b) and to $\Gamma_{a,b}/\Gamma_{c,1} = 1$ (panel c).

Regarding $\Phi/\Phi_0 \simeq 1/2$, the approximation given by Eq. (32) (blue stars) is close to the numerically exact result (magenta line) at the smallest values of $\Gamma_{a,b}/\Gamma_{c,1} = 0.5$ and $\Gamma_{c,2}/\Gamma_{c,1} = 2$ on panel a. However, if $\Phi/\Phi_0 \simeq 1/2$, the approximation given by Eq. (32) increases more and more as $\Gamma_{a,b}/\Gamma_{c,1}$ is increased (see panels b and c), whereas the numerically exact result shows the opposite trend (*i.e.* reduction as $\Gamma_{a,b}/\Gamma_{c,1}$ increases). The identical values for $\Gamma_{c,1} = \Gamma_{c,2}$ on panels d, e and f yield even stronger deviations in perturbation theory because the numerically exact calculations show that $I_c(1/2) = 0$ is vanishingly small at $\Phi/\Phi_0 = 1/2$, whatever $\Gamma_{a,b}/\Gamma_{c,1}$, while the approximation (32) is far above the exact numerical result of $\Phi/\Phi_0 \simeq 1/2$. The numerically exact calculation showing $I_c(1/2) = 0$ if $\Gamma_{c,1} = \Gamma_{c,2} = 0$ and $\Phi/\Phi_0 = 1/2$ is the result of $\Gamma_{c,eff} = 0$ with these parameters [see Eq. (22) in the text of the paper].

Figure 1 suggests that the small-$\Gamma_a$ and small-$\Gamma_b$ approximation is more robust at small $\Phi/\Phi_0 \simeq 0$ than at $\Phi/\Phi_0 \simeq 1/2$. A possible interpretation is that deviations from the small-$\Gamma_a$ and small-$\Gamma_b$ perturbative behavior is driven by the $\Phi/\Phi_0 \simeq 1/2$ values, which have thus weaker influence on $\Phi/\Phi_0 \simeq 0$. In addition, Eq. (32) shows breakdown of perturbation theory if $\Gamma_{c,1} = \Gamma_{c,2}$ and $\Phi/\Phi_0 = 1/2$ in the sense of production of a diverging $I_c(\Phi/\Phi_0)$ which is not there at $\Phi/\Phi_0 = 0$, see Eq. (31).

We note that $\Gamma_{c,eff} = \mathscr{D}(\Phi/\Phi_0)$, where $\Gamma_{c,eff}$ is defined by Eq. (22) in the text of the paper, and $\mathscr{D}(\Phi/\Phi_0)$ is defined by the above Eq. (24). Then, emergence of an ABS at zero energy for $\Gamma_a = \Gamma_b = 0$, $\Gamma_{c,1} = \Gamma_{c,2}$ and $\Phi/\Phi_0 = 1/2$ is compatible with the breakdown of perturbation theory obtained for these parameters.

Now, we present figure 2 showing similar plots as figure 1 but now with the coupling constants $\Gamma_a$, $\Gamma_b$, $\Gamma_{c,1}$ and $\Gamma_{c,2}$ parameterized according to Eqs. (25)-(28) in the text of the paper.

The range of the control parameter $\gamma/\Delta$ (from $\gamma/\Delta = -0.25$ on figure 2a to $\gamma/\Delta = 0.25$ on figure 2f) is similar to the numerical calculations at finite voltage $V$ presented in the text of the paper, where the ratio $\gamma/\Delta$ goes from $-0.25$ to 0.3. A small dependence of the critical current $I_c(\Phi/\Phi_0)$ on the reduced flux $\Phi/\Phi_0$ is found on panel a. This is because the loop is disconnected if $\gamma/\Delta = -0.3$ is used, *i.e.* $\gamma/\Delta = -0.3$ implies $\Gamma_{c,1}/\Delta = 0$ in Eq. (27) in the text of the paper. The amplitude of the modulations of $I_c(\Phi/\Phi_0)$ increases as $\gamma/\Delta$ is increased, because both arms become more strongly to the loop.

Changing $\gamma$ from $\gamma/\Delta = -0.25$ to $\gamma/\Delta = 0.25$ in figure 2 of the Supplemental Material shows that both the approximation given by Eq. (29) and the numerically exact values of $I_c(\Phi/\Phi_0)$ are insensitive on $\gamma/\Delta$ if the value $\Phi/\Phi_0 = 1/2$ of the reduced flux is used. This is because Eqs. (27)-(28) in the text of the paper imply that $\Gamma_{c,eff}$ [see Eq. (22) in the text of the paper] is independent on $\gamma/\Delta$ if $\Phi/\Phi_0 = 1/2$.

## III. ROBUSTNESS OF THE INVERSION WITH RESPECT TO CHANGING $\gamma/\Delta$.

In this section, we show that the inversion is robust with respect to the weak-to-strong Landau-Zener tunneling crossover. We first consider the connection between the Floquet spectrum and the quartet current in the regime of strong Landau-Zener tunneling (see section III A), and next consider the entire range of $\gamma/\Delta$ in section III B.

### A. Robustness of the connection between the quartet current and the Floquet spectra

This subsection deals with establishing the robustness of the connection between the quartet current and the Floquet spectra in the regime of strong Landau-Zener tunneling.

To further illustrate this point, let us now consider figure 3 which is analogous to figure 6 in the paper, but for $\gamma/\Delta = -0.25$ instead of $\gamma/\Delta = 0.3$. It was shown in section IV of the paper that the parameter $\gamma/\Delta = -0.25$ yields strong Landau-Zener tunneling (see figure 4-c1-c2 in the paper) while the previous $\gamma/\Delta = 0.3$ and $\Phi/\Phi_0 = 0$ was representative of weak Landau-Zener tunneling (see figure 4-a1-a2 in the paper).

We first note that the critical current $I_{q,c}(eV/\Delta, \Phi/\Phi_0)$ plotted as a function of $eV/\Delta$ is irregular at strong Landau-Zener tunneling, *i.e.* for $\gamma/\Delta = 0.3$, $\Phi/\Phi_0 = 0$ on figure 6d in the paper, or $\gamma/\Delta = -0.25$, $\Phi/\Phi_0 = 0$ on figure 3b, or $\gamma/\Delta = -0.25$, $\Phi/\Phi_0 = 1/2$ on the following figure 3d.

We speak now about the "extrema" in the Floquet spectra at "strong Landau-Zener tunneling", instead of "avoided crossings" which is reserved to "weak Landau-Zener tunneling". In spite of irregularities in the location of the extrema of the Floquet spectrum on the voltage axis, figures 3-a-b (for $\gamma/\Delta = -0.25$ and $\Phi/\Phi_0 = 0$) and figures 3-c-d (for $\gamma/\Delta = -0.25$ and $\Phi/\Phi_0 = 1/2$) reveal a series of coincidence between the extrema in the Floquet spectra (panels a and c) and the minima in the quartet current (panels b and d) in the regime of strong Landau-Zener tunneling.

### B. Robustness of the inversion

Now, we comment in this subsection on figure 4 demonstrating robustness of the inversion with respect to varying

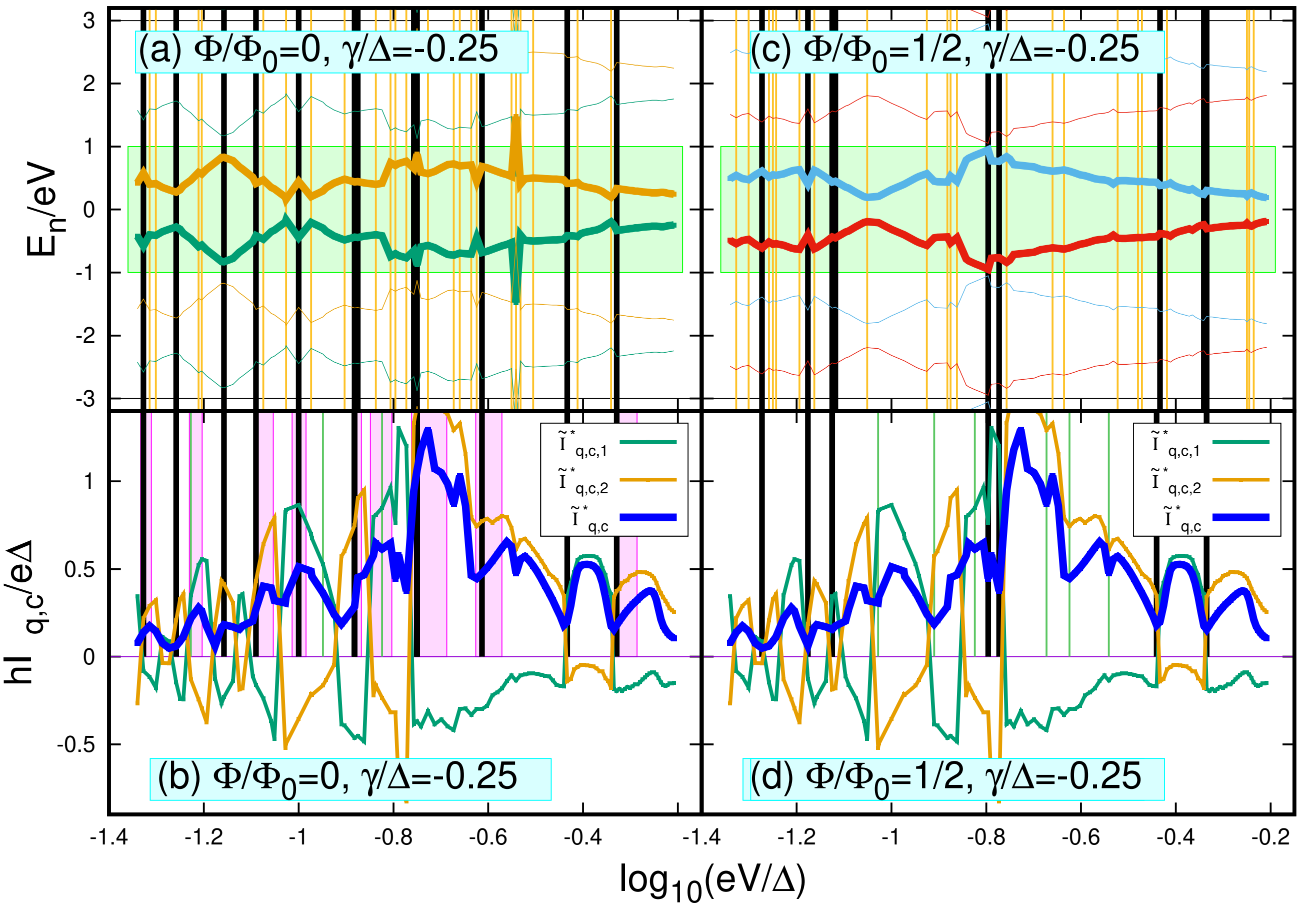


FIG. 3. This figure is similar to figure 6 in the paper, but now with $\gamma/\Delta = -0.25$.

$\gamma/\Delta$ from weak ($\gamma/\Delta = 0.3$ and $\Phi/\Phi_0 = 0$) to strong ($\gamma/\Delta = -0.25$ and $\Phi/\Phi_0 = 0$) Landau-Zener tunneling.

Specifically, panels a-l of figure 4 show the critical current $I^*_{q,c}$ (on the $y$-axis) as a function of reduced voltage $eV/\Delta$ (on the $x$-axis). The values of $\gamma/\Delta$ [see Eqs. (25)-(28) in the paper] range from $\gamma/\Delta = -0.25$ (panel a) to $\gamma/\Delta = 0.3$ (panel l). The black and magenta lines correspond to reduced fluxes $\Phi/\Phi_0 = 0$ and $\Phi/\Phi_0 = 1/2$ respectively, as indicated on the figure. Inversions between $\Phi/\Phi_0 = 0$ and $\Phi/\Phi_0 = 1/2$ [*i.e.* $I^*_{q,c}(eV/\Delta, 0) < I^*_{q,c}(eV/\Delta, 1/2)$] appear at the specific $eV/\Delta$-values shown by the magenta shading.

The inversion between $\Phi/\Phi_0 = 0$ and $\Phi/\Phi_0 = 1/2$ emerges on all panels corresponding to $\gamma/\Delta$ between $\gamma/\Delta = -0.25$ and $\gamma/\Delta = 0.3$.

A simple mechanism for the inversion operates in the limit of weak Landau-Zener tunneling (see sections II B and V in the paper) but figure 4 tells that the inversion is also there if $\gamma/\Delta = -0.25$ at strong Landau-Zener tunneling. The inversion is even favored upon reducing $\gamma/\Delta$ from 0.3 to $-0.25$. It turns out that $S_{c,1}$ is disconnected from the dot if $\gamma/\Delta = -0.3$ [see Eqs. (25)-(28) in the paper]. The resulting $\tilde{I}^*_{q,c}(eV/\Delta)$ is then trivially independent on $\Phi/\Phi_0$ at this specific value $\gamma/\Delta = -0.3$. The identical values $\tilde{I}^*_{q,c}(eV/\Delta, 0) = \tilde{I}^*_{q,c}(eV/\Delta, 1/2)$ at $\Phi/\Phi_0 = 0$ or $\Phi/\Phi_0 = 1/2$ tend to favor emergence of the inversion for $\gamma/\Delta \gtrsim -0.3$.


[1] M. L. Goldberger and K. M. Watson, *Collision Theory*, John Wiley and Sons, New York (1964).

[2] A. Prêtre, H. Thomas, and M. Büttiker, *Dynamic admittance of mesoscopic conductors: Discrete-potential model*, Phys. Rev. B **54**, 8130, (1995).

[3] L. Arrachea and M. Moskalets, *Relation between scattering-matrix and Keldysh formalisms for quantum transport driven by time-periodic fields*, Phys. Rev. B **74**, 245322, (2006).

[4] R. Mélin, R. Danneau, K. Yang, J.-G. Caputo, and B. Douçot, *Engineering the Floquet spectrum of superconducting multiterminal quantum dots*, Phys. Rev. B **100**, 035450 (2019).

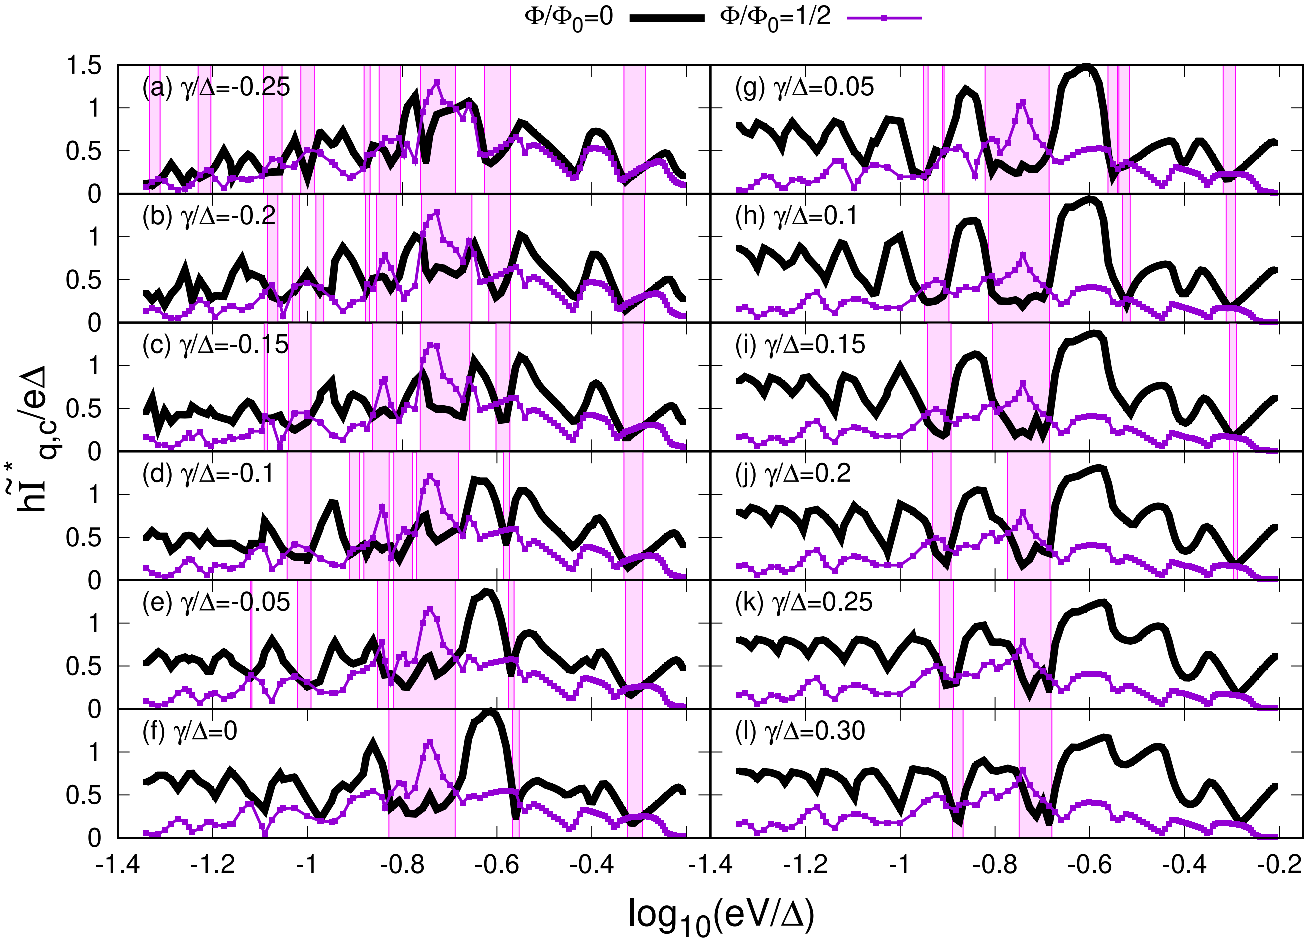


FIG. 4. The figure shows the critical quartet current $\tilde{I}^*_{q,c}(eV/\Delta,\Phi/\Phi_0)$ as a function of reduced voltage $eV/\Delta$ for $\Phi/\Phi_0=0$ (black lines) and $\Phi/\Phi_0=1/2$ (magenta lines). The magenta shading corresponds to the inversion, *i.e.* to $\tilde{I}^*_{q,c}(eV/\Delta,0)<\tilde{I}^*_{q,c}(eV/\Delta,1/2)$.
